# Supplementary material for: UPAR: Unified Pedestrian Attribute Recognition and Person Retrieval
Source: arXiv:2209.02522 source file (2022-09-06)
Supplement: Supplementary file 1 [file X_supplementary.tex]

\appendix
% --- PDF will be split by an editor (e.g. macOS preview), so need to restart from page 1
\setcounter{page}{1}

% --- repeat the title (AT: haven't found a more elegant way to do this...)
\twocolumn[
\centering
\Large
\textbf{UPAR: Unified Pedestrian Attribute Recognition and Person Retrieval} \\
\vspace{0.5em}Supplementary Material \\
\vspace{1.0em}
] %< twocolumn
\appendix

\input{sec/0_acronyms}

\section{Further Evaluation}

\subsection{Training Setup}
We train our models using PyTorch 1.11 and CUDA 11.3.
To speed up the trainings, we leverage adaptive mixed precision scaling of the models' trainable parameters.
The experiments were done on a server with NVIDIA GeForce RTX 3090 GPUs.

\subsection{Additional CV Results}
For simplicity, we provide additional results based on split 0 of the \acrshort{cv} evaluation protocol and with \acrshort{cnb} as backbone in \cref{tab:upar_cv_ext}.
It is observable that applying the AdamW optimizer directly to the baseline does not lead to an improvement in contrast to using it in conjunction with an optimized and regularized model.
Besides, computing the EMAs of the model's parameters deteriorates all metrics.
Due to the limited amount of training data, it was hardly possible for the training to converge.
Furthermore, the results are clearly influenced by the training batch size.
In this case, halving the batch size from 64 to 32 decreases, e.g., the F1 score by 1.4 percentage points.
Regarding dropout, the maximum is reached for a dropout rate of 0.7 for three of the four metrics.
Similar to the batch size, significant differences occur for small changes in the dropout rate parameter.
In addition, the influence of the loss smoothing parameter $\alpha$ is shown.
The results indicate that higher values for $\alpha$ are beneficial concerning the metrics of \acrshort{par}.
I.e., when optimizing the model for attribute recognition, an even larger $\alpha$ might further increase the results.
However, person retrieval suffers.
A possible explanation is that the model gets underconfident about attributes at a certain point.
As a result, correct matches may obtain a larger distance during retrieval and appear in later positions.
Due to a fixed threshold, this is not an issue for \acrshort{par}.

\begin{table}[t]
\centering
	\resizebox{\linewidth}{!}{ %< auto-adjusts font size to fill line
		\begin{tabular}{@{}l|cccc@{}}%
			\toprule%
			Approach & mA & F1 & mAP & R-1 \\%
			\midrule%
			Baseline (B) & 68.5 & 74.6 & 6.5 & 5.7 \\%
			\midrule%
			B + AdamW & 68.4 & 73.4 & 6.2 & 5.5 \\%
			\midrule%
			B + EMA & 65.2 & 73.3 & 5.3 & 5.0 \\%
			\midrule%
			B + Batch size (BS) 16 & 67.8 & 73.4 & 5.5 & 5.1 \\%
			B + BS 32 & \textbf{68.5} & 73.2 & 5.7 & 5.0\\%
			B + BS 64 & \textbf{68.5} & \textbf{74.6} & \textbf{6.5} & \textbf{5.7} \\%
			B + BS 128 & 67.8 & 73.2 & 6.0 & 5.3 \\%
			\midrule%
			B + BS 64 + Dropout (DO) 0.5 & 67.4 & 74.9 & 7.0 & 6.7 \\%
			B + BS 64 + DO 0.6 & 67.9 & \textbf{76.0} & 7.3 & 7.2 \\%
			B + BS 64 + DO 0.7 & \textbf{68.2} & 75.7 & \textbf{7.6} & \textbf{7.5} \\%
			B + BS 64 + DO 0.8 & 67.3 & 75.0 & 7.1 & 6.7 \\%
			B + BS 64 + DO 0.9 & 66.3 & 73.5 & 6.8 & 6.0 \\%
			\midrule%
			B + BS 64 + DO 0.7 + Label smoothing (LS) 0.05 & 68.4 & 76.0 & 8.1 & 7.6 \\%
			B + BS 64 + DO 0.7 + LS 0.1 & 68.5 & 76.2 & \textbf{8.2} & \textbf{7.7} \\%
			B + BS 64 + DO 0.7 + LS 0.15 & \textbf{68.7} & \textbf{76.3} & 8.0 & 5.2\\%
			\bottomrule%
		\end{tabular}%
	}% \resizebox
	\caption{
		\textbf{UPAR CV} -- Ablation Study
	} % \caption
	\label{tab:upar_cv_ext}%
\end{table}

\section{Further Evaluation}

\subsection{Training Setup}
We train our models using PyTorch 1.11 and CUDA 11.3.
We leverage adaptive mixed precision scaling of the models' trainable parameters to speed up the training.
The experiments were done on a server with NVIDIA GeForce RTX 3090 GPUs.

\subsection{Additional CV Results}
For simplicity, we provide additional results based on split 0 of the \acrshort{cv} evaluation protocol and with \acrshort{cnb} as backbone in \cref{tab:upar_cv_ext}.
It is observable that applying the AdamW optimizer directly to the baseline does not lead to an improvement in contrast to using it in conjunction with an optimized and regularized model.
Besides, computing the EMAs of the model's parameters deteriorates all metrics.
Due to the limited amount of training data, it was hardly possible for the training to converge.
Furthermore, the results are clearly influenced by the training batch size.
In this case, halving the batch size from 64 to 32 decreases, e.g., the F1 score by 1.4 percentage points.
Regarding dropout, the maximum is reached for a dropout rate of 0.7 for three of the four metrics.
Similar to the batch size, significant differences occur for small changes in the dropout rate parameter.
In addition, the influence of the loss smoothing parameter $\alpha$ is shown.
The results indicate that higher values for $\alpha$ are beneficial concerning the metrics of \acrshort{par}.
I.e., when optimizing the model for attribute recognition, an even larger $\alpha$ might further increase the results.
However, person retrieval suffers.
A possible explanation is that the model gets underconfident about attributes at a certain point.
As a result, correct matches may obtain a larger distance during retrieval and appear in later positions.
Due to a fixed threshold, this is not an issue for \acrshort{par}.

\begin{table}
\centering%
%\resizebox{\linewidth}{!}{ %< auto-adjusts font size to fill line
\begin{tabular}{@{}l|l@{}}%
\toprule%
Category & Attribute \\%
\midrule
\multirow{3}{*}{Age} & Young \\%
    & Adult \\%
    & Elderly \\%
\midrule%
Gender & Female \\%
\midrule%
\multirow{3}{*}{Hair length} & Short \\%
    & Long \\%
    & Bald \\%
\midrule%
Upper-body clothing length & Short \\%
\midrule%
\multirow{12}{*}{Upper-body clothing color}%
    & Black \\%
    & Blue \\%
    & Brown \\%
    & Green \\%
    & Grey \\%
    & Orange \\%
    & Pink \\%
    & Purple \\%
    & Red \\%
    & White \\%
    & Yellow \\%
    & Other \\%
\midrule%
Lower-body clothing length & Short \\%
\midrule%
\multirow{12}{*}{Lower-body clothing color}%
    & Black \\%
    & Blue \\%
    & Brown \\%
    & Green \\%
    & Grey \\%
    & Orange \\%
    & Pink \\%
    & Purple \\%
    & Red \\%
    & White \\%
    & Yellow \\%
    & Other \\%
\midrule%
\multirow{2}{*}{Lower-body clothing type}%
    & Trousers\&Shorts \\%
    & Skirt\&Dress \\%
\midrule%
Accessory Backpack & Backpack \\%
\midrule%
Accessory Bag & Bag \\%
\midrule%
\multirow{2}{*}{Accessory Glasses}% 
    & Normal \\%
    & Sun \\%
\midrule%
Accessory Hat & Hat \\%

\bottomrule
\end{tabular}%
\caption{Attribute annotations included in the \acrshort{upar} dataset.}
\label{tab:upar_atts}
\end{table}
\section{UPAR Attributes}
\cref{tab:upar_atts} contains a complete list of the 40 annotated attributes and their 12 categories.
All attributes are binary, i.e., a value of 0 denotes the absence and a value of 1 the presence of an attribute, respectively.
For attributes such as clothing lengths or gender, the value 0 stands for the opposite meaning, i.e., male persons or long clothing.
Please note that we only consider the perceived visual appearance of people and thus consider gender as binary, even though persons might be non-binary.

\section{UPAR Annotation Process}
In this section, we describe in detail the annotation process followed by our annotators and the challenges encountered.
In order to deliver the \acrshort{upar} dataset, supplementary annotations for PA100k~\cite{liu2017hydraplus} (lowerBodyClothingColor and upperBodyClothingColor), PETA~\cite{deng2014pedestrian} (lowerBodyClothingLength) and RAPv2~\cite{8510891} are required. 
The annotators are informed that the datasets are composed of camera shots of people from different perspectives, exposure ratios, and measures of crowd intensity. Individuals may appear in multiple shots. The attribute classification is performed for each frame individually, i.e., when describing the person's attributes of the same person in different frames, only the visible information of the frame to be classified is considered.
Thus, different values of the considered person attributes can be assigned to the same person in different frames depending on the lighting, shadows cast by objects or people, or the clothing area visible in the frame.

\subsection{Annotation of UpperBodyClothingColor and LowerBodyClothingColor}

For each frame, a primary person is selected whose body area is divided into the two areas up the hips (Upper+body) and down the hips (Lower-body).
The clothing for the upper-body and lower-body regions is classified by determining the color class for the UpperBodyClothingColor and LowerBodyClothingColor attributes, respectively. 
The color classes are divided into unique color classes (black, white, grey, red, blue, yellow, orange, green, purple, pink, purple), a collection class (other), and a class for missing assignments (unknown).

\subsubsection*{Selection of the primary person}
Before attribute classification, the primary person of the frame is determined. If only one person is in the frame, this person can be uniquely determined as the primary person. However, if there is more than one person in the frame, the one mapped as centrally as possible and with the least amount of overlap by objects or other persons is determined as the primary person.
In the case that no primary person can be determined unambiguously, the clothing of both body areas is classified as unknown.

\subsubsection*{Selection of the primary color}
The primary color of the clothing is the color class whose share of the represented pixel area corresponds to at least 50\%. For example, different shades of blue count together in the share of the color class blue.
Colors that cannot be unambiguously assigned to the unique color classes are assigned to the other collection class. These include metallic colors and the color beige.
If the corresponding body area of the primary person is not represented in the frame or if the primary person is represented in false colors, e.g., grayscale, an assignment to the class unknown is made.

\subsubsection*{Description of further color classes}
If (at least) one other color class exists, whose area share is at least 10\% of the pixel area, this is classified by setting the flag mixture.

\subsubsection*{Special cases}
If no unique primary color can be assigned to the primary person, for example, because the clothing is uniformly striped or the clothing is colorfully dotted, the frame is classified by the combination other + mixture.
Please note that we do not use the mixture class so far.
Infants are not selected as primary persons. Instead, the accompanying person is selected as the primary person despite possible occlusion by the child.

\subsection{Annotation of LowerBodyClothingLength}

For each frame, a primary person is selected (analogous to above) whose body area is divided into the two areas up the hips (Upper-body) and down the hips (Lower-body).
The clothing in the lower body region is classified by determining the length class for the LowerBodyClothingLength attribute. 
The length classes can be divided into two unique classes (long, short) and one for missing assignments (unknown).

\subsubsection*{Selection of the primary person}
Before attribute classification, the primary person of the frame is determined. If only one person is in the frame, this person can be uniquely determined as the primary person. However, if there is more than one person in the frame, the one that is mapped as centrally as possible and with the least amount of overlap by objects or other persons is determined as the primary person.
In case no primary person can be determined unambiguously, the clothing of both body parts is classified as unknown.

\subsubsection*{Selection of the length class}
The lower body clothing is assigned the length class long if at least the thighs and the knees are clothed. 
The length class short is assigned if parts of the thigh or knee area are not clothed.
If the lower-body of the primary person is not entirely shown on the frame and thus no clear assignment to the classes, long or short, is possible, the underwear is assigned to the class unknown.

\subsubsection*{Special cases}
If only the lower-body clothing of one leg is wholly mapped on the frame, it is assumed that this is representative of the entire lower clothing.

\subsection{Annotation of Age}
For each frame, a primary person is selected (analogous to above). If the person is not clearly underaged (child, teenager) or clearly an adult or elderly, the attribute is set to unknown.

\subsection{Annotation of the hair length}
For each frame, a primary person is selected (analogous to above). 
In this case, the annotator should answer the following questions:
\begin{enumerate}
    \item short: Are this person's hair shorter than shoulder length?
    \item long: Is this person's hair at least shoulder length?
    \item bald: Is this person (partly) bald?
    \item unknown: is it for some reasons not clear? (hat, low-resolution, etc.)
    \item Are multiple of the above true? E.g., a bald patch fits both bald and short (or even long).
\end{enumerate}

\subsection{Annotation of Glasses}
For each frame, a primary person is selected (analogous to above). 
In this case, the annotator should answer the following questions:
\begin{enumerate}
    \item glasses: Can you recognize if this person is wearing glasses?
    \item sunglasses: If so, are those sunglasses?
    \item unknown: difficult to tell / the person looks away from the camera
\end{enumerate}

\subsection{Shortcuts for fast annotation}
The whole annotation process is performed on our annotation tool. 
In order to improve annotation speed, we design extra classification shortcuts for this task. 
First, based on the available color labels provided by Market-1501-attributes, PETA, and RAPv2, we analyze the distribution of color occurrences and determine the most common colors. 
Second, in dialogue with our annotator team, we analyzed the ergonomy of different solutions to speed up the annotation process without inducing mistakes due to misuse of the software. We found out that image-based annotation does necessarily require the use of a mouse. If designed correctly, shortcuts divided on both hands result in more efficient workflows and more comfort for the user.  
The final solution results in using the left-hand for changing images (\textit{a - d}) and setting the annotation status (\textit{r} for review, \textit{f} for finished). The right hand is used for classification. Given a Numpad and the use of five fingers, the standard positions for the fingers are for the right hand:  \textit{thumb free, four, eight, six, enter}. We, therefore, associate the most used colors with the most used keys. As shown in~\cref{fig:shortcuts},
we associate color codes with the color annotation of upperBodyColor and lowerBodyColor. The upperBodyColor is annotated with the first code, and the lowerBodyColor is annotated with the second code. For instance, the sequence \textit{5} and \textit{88} result in annotating upperBodyColor-white and lowerBodyColor-black. The color matrix~\cref{fig:shortcuts} is printed and learned from each annotator. After a few hours, this method results in the annotation of around 12-20 frames per minute (for both upperBodyColor and lowerBodyColor) when annotating an image for the first time. Around 6-12 frames are validated per minute.

\begin{figure}[t]
\begin{center}
% \begin{overpic} 
% [width=\linewidth]
% {example-image-a}
% \end{overpic}
\includegraphics[width=0.75\linewidth]{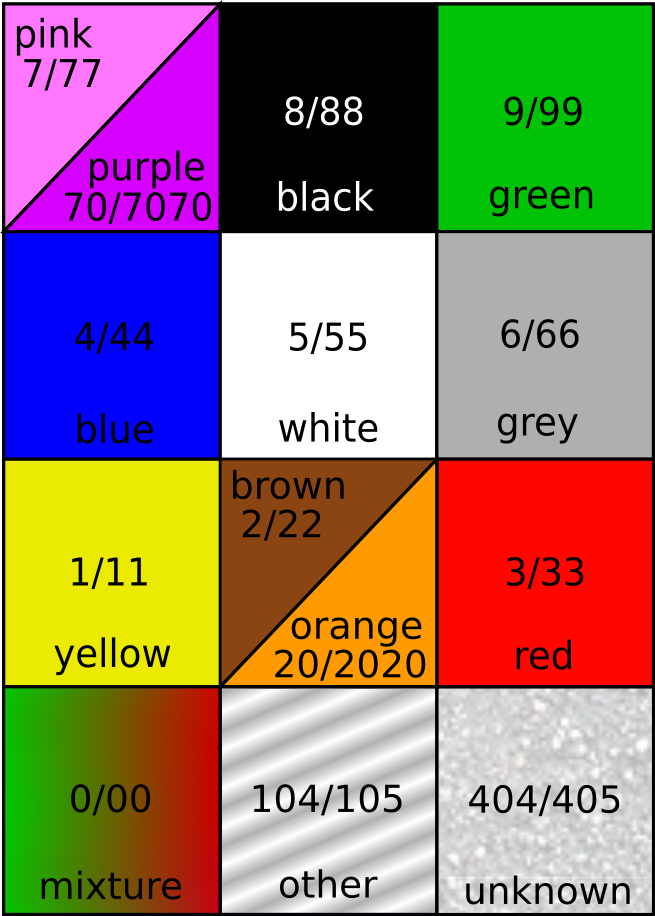}
%\vspace{-0.3cm}
\end{center}
\caption{
\textbf{Annotation Shortcuts -- }
Shortcuts keys designed to improve annotation speed. Given a numpad and the use of five fingers, we associate the most often used keys with the most common colors. Standart position for the finger are for the right hand:  \textit{thumb free, four, eight, six, enter}.  The upperBodyColor is annotated with the first code, the lowerBodyColor is annotated with the second code. For instance, the sequence \textit{5} and \textit{88} result in annotating upperBodyColor-white and lowerBodyColor-black.
}

\label{fig:shortcuts}
%\vspace{-0.3cm}
\end{figure}

\subsection{Validation process}

A team of annotators performs the validation process. Two types of errors can occur during the classification process:

\begin{enumerate}
    \item \textbf{Operator errors} When classifying thousands of frames, some frames will inevitably cause the classification software to operate incorrectly, for example, by double-assigning a primary color class.
    \item \textbf{Perceptual inconsistency}
Color perception depends on other factors besides image information. These include external factors such as room lighting or monitor settings and factors internal to the person, such as the perception of contrast information or an undetected color vision deficiency.
As a result, annotators sometimes assign the same frame to different color classes. Thus, the randomization of the frame order and the resulting division of a frame series into different sequences results in inconsistent classifications, especially for frames with colors that lie at the boundary between multiple color classes.
\end{enumerate}

To maintain consistency, each frame sequence is checked following the classification process according to the dual control principle by an annotator (validator) who has not previously classified the frame sequence. In this process, operating errors are detected and corrected directly by the validator. 
To resolve the perceptual inconsistency, a database of inconsistent frames was created. There, through the participation of all team members, a unique and consistent classification was determined for each corresponding frame. Furthermore, by regularly updating and viewing the database, it was possible to ensure that all annotators consistently classified the individual frames of the different frame series.
 
The annotators' tasks thus include classifying the frame sequences assigned to them and checking each other in the validation process while constantly cooperating to maintain classification consistency.

\subsection{Final step}
\begin{table}
\centering
%\resizebox{\linewidth}{!}{ %< auto-adjusts font size to fill line
\begin{tabular}{@{}l|l|l|l@{}}
\toprule%
\multirow{2}{*}{Partition in pickle file} & \multicolumn{2}{c|}{Generalization} & \multirow{2}{*}{Specialization} \\%
& CV split & LOO split \\% 
\midrule%
0 & - & - & 0 \\%
1 & 0 & - & - \\%
2 & - & 0 & - \\%
3 & 1 & - & - \\%
4 & - & 1 & - \\%
5 & 2 & - & - \\%
6 & - & 2 & - \\%
7 & 3 & - & - \\%
8 & - & 3 & - \\%
\bottomrule
\end{tabular}
%} % \resizebox
\caption{
\textbf{\acrshort{upar} splits} -- Nine different partitions are included in the dataset pickle file. The first column denotes the index in the pickle file and the second and third column stands for the partition number analogous to those used in the paper for the generalization experiments. Partition 0 in the pickle file corresponds to the specialization split, i.e., data from all sub-datasets is used for training and evaluation.
} % \caption
\label{tab:upar_splits_all}
%\vspace{-0.3cm}
\end{table}
We construct the final dataset by merging the sub-datasets with our annotations into a pickle file.
We extract the labels for the UPAR attributes for each dataset from either the original annotations or our annotations.
Some colors are not annotated for all datasets.
For instance, the Market-1501 dataset has fewer colors compared to RAPv2.
To handle this, we set the corresponding attribute labels to \textit{not present} for the whole dataset since other colors are assigned to the images.
Furthermore, please note that we discard images that were labeled as unknown since relevant attributes might not be visible in the images.
Mainly the PA100k dataset contains many images with, \eg, heavily occluded persons or only partly visible persons.
Finally, we create a pickle file that includes all the necessary information. 
The file (UPAR/dataset.pkl), as well as a python class to load the file as pytorch dataset (UPAR/UPAR.py) are also included in the supplementary material.
To use it, the original sub-datasets must be extracted in a directory, \eg, \textit{datasets/Market-1501}, \textit{datasets/PA100k}, etc.
In contrast to the generalization splits presented in the paper, the pickle file contains nine different partitions which correspond to the different training sets.
\cref{tab:upar_splits_all} shows the differences between the partitions and denotes the connection to the generalization and specialization splits.
